# Supplementary material for: Causal inference for social network formation
Source: arXiv:2604.17952 source file (2026-04-20)
Supplement: Supplementary file 1 [file B_additionalplots.tex]

\section{Additional plots}
\label{sec:additionalplots}

\begin{figure}[H]
    \caption{Permutation distribution of placebo estimates}
    \label{fig:permutationplacebo}
\begin{center}
\vspace{10pt}

\includegraphics[width = \textwidth]{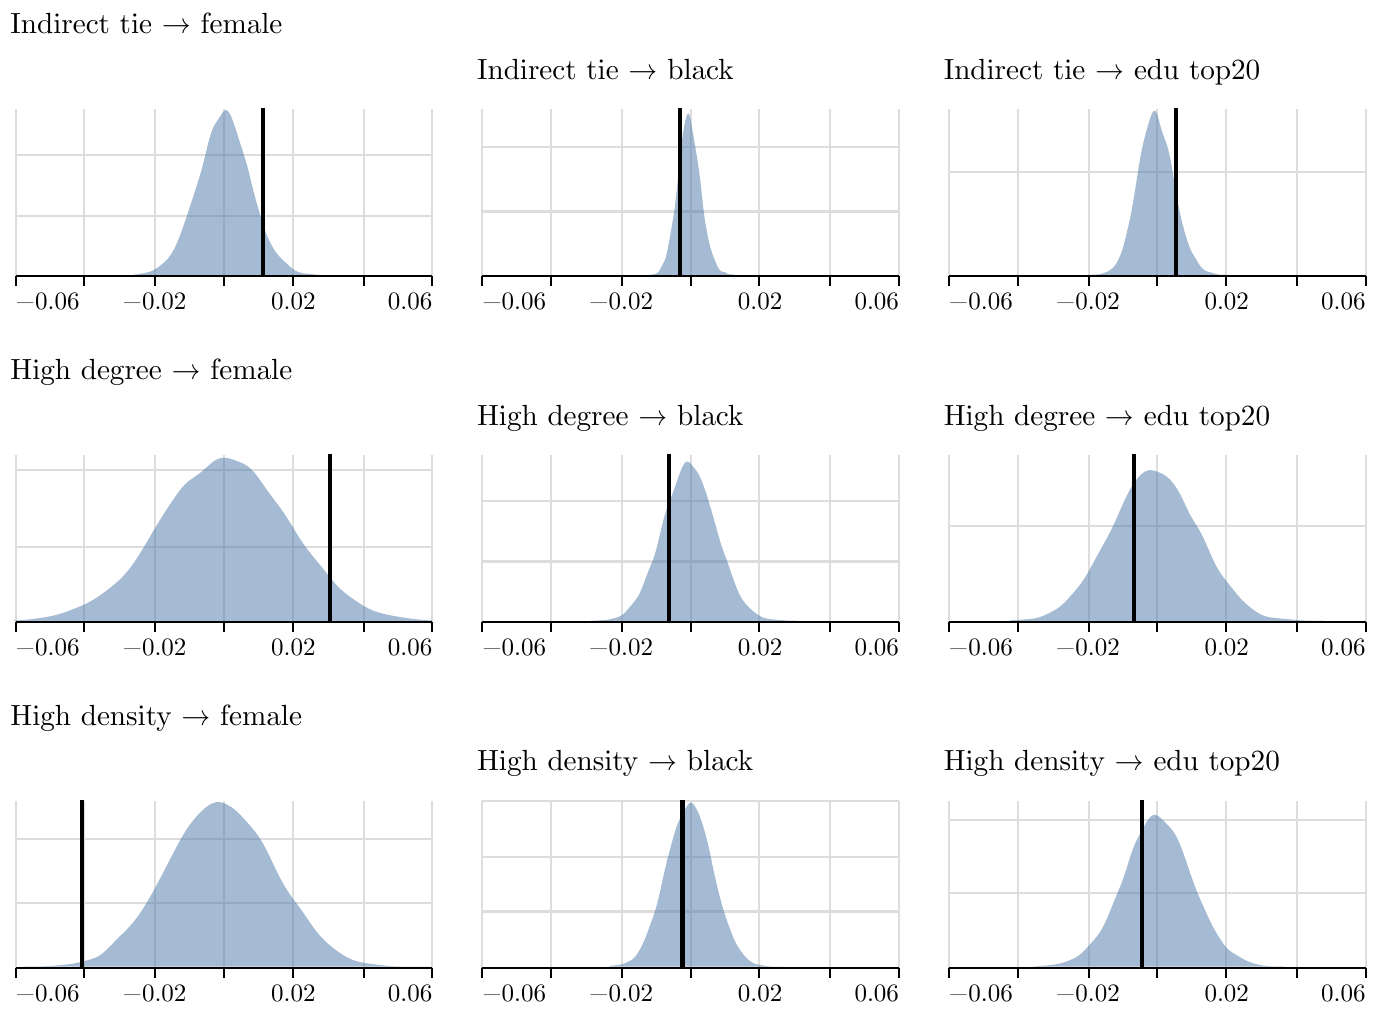}\\[12pt]
\end{center}
\footnotesize
\textit{Notes:} These figures show the distribution of counterfactual estimates of placebo regressions under 10,000 permutations of new hires within offices. The black lines indicate the actual point estimate. The quantile of the point estimate in the randomization distribution corresponds to the p-values shown in \autoref{tab:placeboestimates}.
\end{figure}

\clearpage
\begin{figure}[H]
\caption{Permutation distribution of estimates}
\label{fig:permutationinference}
\vspace{10pt}
\includegraphics[width = \textwidth]{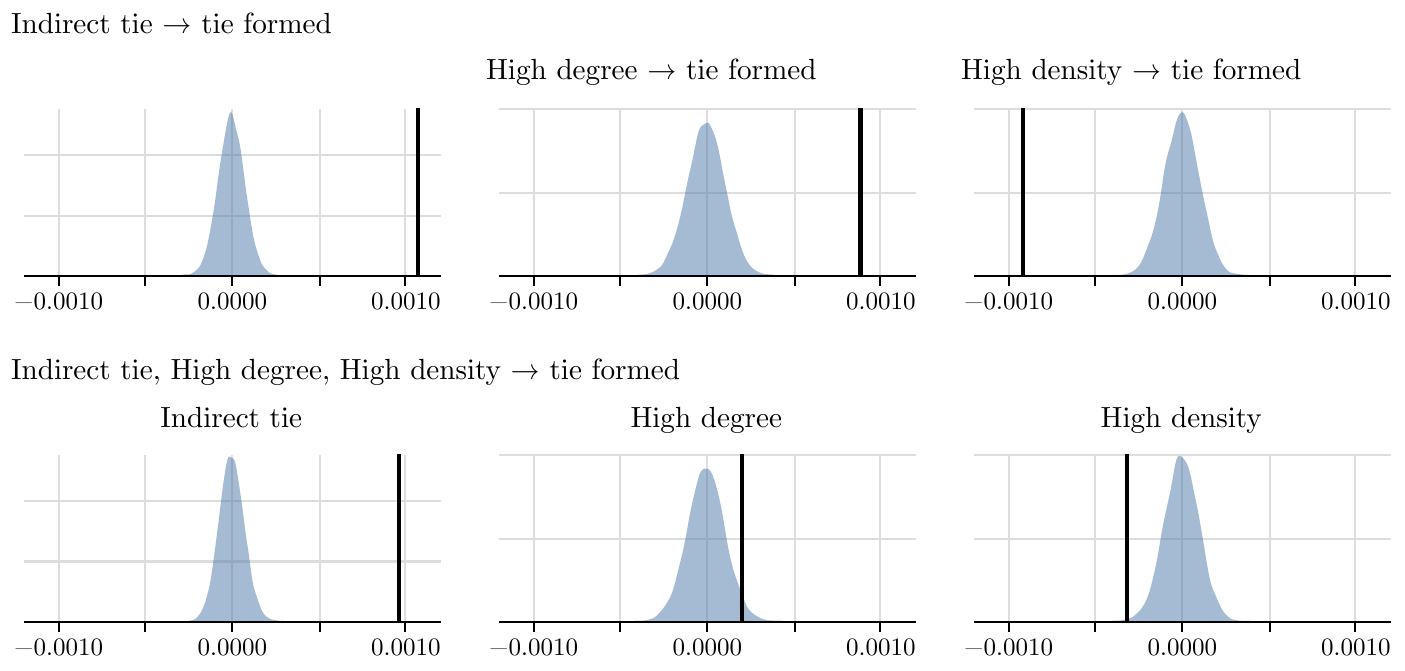}\\[12pt]
\footnotesize
\textit{Notes:} These figures show the distribution of counterfactual estimates under 10,000 permutations of new hires within offices. The black lines indicate the actual point estimate. The quantile of the point estimate in the randomization distribution corresponds to the p-values shown in \autoref{tab:effectestimates}.\\[12pt]

\caption{Permutation distribution of estimates, continuous regressors}
\label{fig:permutationinferencecontinuous}
\vspace{10pt}
\includegraphics[width = \textwidth]{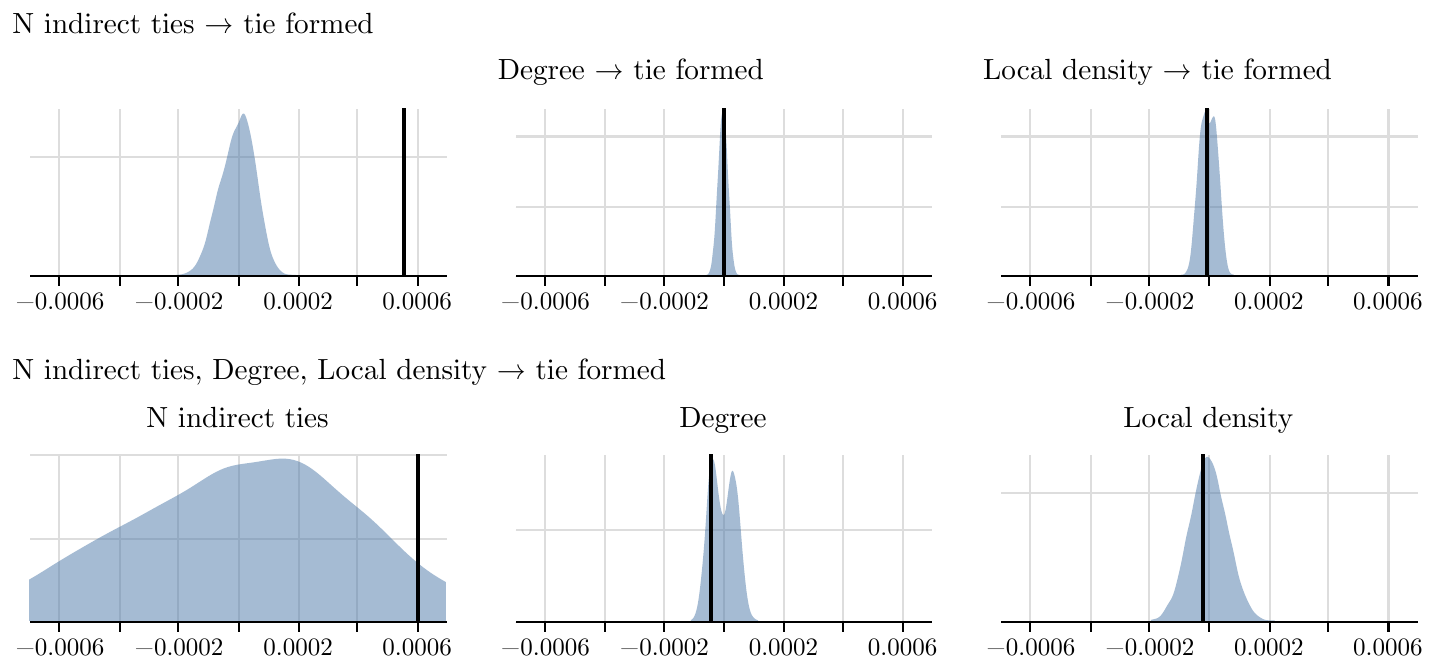}\\[12pt]
\footnotesize
\textit{Notes:} These figures show the distribution of counterfactual estimates under 10,000 permutations of new hires within offices. The black lines indicate the actual point estimate. The quantile of the point estimate in the randomization distribution corresponds to the p-values shown in \autoref{tab:continuousestimates}.
\end{figure}
