# Supplementary material for: Causal inference for social network formation
Source: arXiv:2604.17952 source file (2026-04-20)
Supplement: Supplementary file 2 [file C_additionaldiscussion.tex]

\section{Additional discussion}
\label{sec:additionaldiscussion}

\paragraph{Review: Causal inference in RCTs}
The framework as stated in \autoref{sec:setup} fairly abstract. To fix ideas and to motivate our estimands and estimators below, it is useful to relate this framework to the conventional setting of causal inference in randomized controlled trials with binary treatments \citep{imbens2015causal}.

This conventional setting describes the effect of binary treatments in the absence of interference (spillovers). There is a vector of outcomes $Y$, and a vector of treatments $D$, and the two are related by the causal relationship $Y = g(D)$.
The structural function $g$ (like the function $f$ in the network setting) describes potential (or counterfactual) outcomes. 
Under the assumption of {no interference} (also known as stable unit treatment effects, which is a form of {exclusion restriction}), $Y_j$ only depends on $D_j$, and it is common to define the {potential outcome} notation $Y^d_j = g(D_1,\ldots, D_{j-1}, d, D_{j+1},\ldots, D_n)$. 
A common object of interest is the {(sample) average treatment effect},
$$
SATE = \tfrac1n \sum_{j} \left(Y^1_j - Y^0_j\right).
$$
Note that this definition of the $SATE$ conditions on unobserved heterogeneity by conditioning on the function $g$.
The potential outcomes $Y^d_j$ are thus non-random, by definition; the only potential source of randomness is the treatment assignment $D$.

Under exogenous random assignment of $D$, the $SATE$ can be estimated without bias using {inverse probability weighting} (IPW).
We can write the IPW estimator of the SATE as follows:
\bals
  \widehat Y^d_j &= Y_j \cdot \frac{\bs 1(D_j = d)}{P(D_j = d)},
  &\widehat{SATE} &= \tfrac1n \sum_{j} \left(\widehat Y^1_j - \widehat Y^0_j\right).
\eals
Suppose that the {support condition} $0<P(D_j = 1)<1$ holds for all $j$.
Under this condition, it is easy to see that the IPW estimator is unbiased, $E\left[\widehat{SATE}\right] = SATE$.

We can furthermore perform {randomization inference} on $\widehat{SATE}$ and related objects: Randomization inference, for testing the null of zero treatment effects, assumes that $Y^1_j = Y^0_j$ for all $j$. Under the no interference condition and this null hypothesis, $g(D)$ is known for all counterfactual treatment assignments $D$. Because the sampling distribution of $D$ itself is known, the sampling distribution of any statistic based on $D$ and $Y$ is therefore known.

If heterogeneity or moderators of treatment effects are of interest, one might furthermore consider variants of the $SATE$ for subsets $\mathcal{I}$ of individuals $i$, where these subsets might be defined based on pre-determined individual covariates.
